# Supplementary material for: Entropy-Stable Model Reduction of One-Dimensional Hyperbolic Systems using Rational Quadratic Manifolds
Source: arXiv:2407.12627 source file (2024-07-17)
Supplement: Supplementary file 1 [file momentumtse.tex]

\section{Momentum-conserving tangent space enrichment}
