# Supplementary material for: Entropy-Stable Model Reduction of One-Dimensional Hyperbolic Systems using Rational Quadratic Manifolds
Source: arXiv:2407.12627 source file (2024-07-17)
Supplement: Supplementary file 3 [file redundancyfree.tex]

\section{Redundancy-free tangent space enrichment}
